# Supplementary material for: Producing a BOSS-CMASS sample with DES imaging
Source: arXiv:1906.01136 source file (2019-06-04)
Supplement: Supplementary file 1 [file appendix2.tex]

\appendix

\section{Stripe82}
\notesj{Here or in Appendix. Stripe82 : We will only use CMASS galaxies in stripe82 as the train sample, therefore it is necessary to confirm that CMASS in stripe82 can represent the whole sample. Stripe 82 is [..] imaged 10 times blah blah. \\
Photometric error is smaller than other region. But Extreme deconvolution can cover that. \\
Compare extreme deconvolution distribution... \\
Number density comparison --> Stripe 82 is a bit higher than other region. How to explain that?
SGC has a bit higher number density because more plate was installed in that region. Stripe82 is one of the covered regions? Check!  \\
}

\iffalse
\section{D$\times$C = D$\times$D = C$\times$C comparison in stripe 82}

% cmass st82 : masked by DES gold mask. 
% cmass randoms : cmass sgc. masked by DES gold mask
\begin{figure}
\includegraphics[width=0.5\textwidth]{./figures/cross_cmass_dmass_st82.pdf}
\caption{Cross angular clustering comparison. DMASS is randomly sampled based on assigned membership probability. Individual DMASS galaxies may not be a member of CMASS.  But a group should have the same property with CMASS. If CMASS=DMASS, their cross correlation should be the same.}
\label{fig:cross_cmass_dmass_st82}
\end{figure}
\fi

\section{ Redshift tails in BOSS CMASS }

	\begin{figure}
	\includegraphics[width=0.5\textwidth]{./figures/cfz_comparison_zcut.pdf}
	\caption{Comparison of galaxy clustering from the CMASS sample in small scales before and after applying z-cuts. BOSS measurement was made from the CMASS galaxies only in the range of $( 0.43 < z < 0.7 )$.
		9.7\% galaxies are discarded by these redshift cuts in SGC. However, DMASS sample is characterized from the CMASS sample in the full redshift range because it is difficult to apply the same redshift cuts to photometric samples.
			This galaxy clustering comparison is in order to make sure the redshift cut won?t affect the clustering signal and bias.
			Black dashed line : CMASS with redshift cuts, Red color : CMASS without redshift cuts.
	}
\label{fig:cfz_comparison_zcut}
\end{figure}

\begin{figure}
\centering
\includegraphics[width=0.45\textwidth]{./figures/plot_distributions_cmass.pdf}

\caption{Comparison of galaxy bias constraints from the CMASS clustering before and after applying z-cuts (top), and the monopole measurements used (bottom) to obtain the top panel. BOSS measurement was made from the CMASS galaxies only in the range of $( 0.43 < z < 0.7 )$. ( blue: cmass, red: cmass with zcut )
}
\label{fig:corr_comparison_monopole}
\end{figure}

\section{ Difference in CMASS SGC and NGC }

\subsection{Modeling in stripe 82 \cmt{will be deleted}}
\subsubsection{Catalog matching and train sample}
{\bf include footprint plot?}Stripe 82 is the region on the celestial equator that the SDSS has imaged over ten times, making coadd optical data two times deeper than single epoch SDSS observations. \REF{Aabazajian 2014}
%Abazajian, K. N., Adelman-McCarthy, J. K., Agüeros, M. A., et al. 2009, ApJS, 182, 543
\REF{Annis 2014}.
%Annis, J., Soares-Santos, M., Strauss, M. A., et al. 2014, ApJ, 794, 120
DES Y1 imaged \cmt{$200\degsqr$} of this region, thereby providing a region where data from the two surveys can be matched.
%This region is suitable for sample matching because the DES footprint is slightly overlapped with SDSS in this region. 
%The stripe 82 is $~270 ~deg^2$ region that covers the region define by $-50 < ra < 59$,  $-1.25 < dec < 1.25$. This region is suitable for sample matching because the DES footprint is slightly overlapped in this region. 
The area of overlap contains \cmt{$13000$} BOSS CMASS galaxies. DES colors and manitudes of CMASS galaxies were obtained by cross-matching to the SDSS CMASS sample using a \cmt{$0.0''$} tolerance.
The matching produces a total of \cmt{12600} CMASS galaxies with clean DES photometry; only $1.5\%$ of the BOSS CMASS galaxies were removed in the overlap region. 

%We use DES Y1 Gold galaxies in \cmt{$0.0 deg^2$} of this overlapped region as train sample. Stars are removed by \verb+MODEST==1+. We also removed bad photometric objects\cmt{details} by DES Y1 Gold flag \verb+FLAGS_GOLD[_GRIZ] == 0+ and the \verb|LSS mask| and gold mask [REF]. \cmt{LSS gold mask description}
%This flag and mask exclude only 1.5 \% of BOSS CMASS galaxies in the overlap region. 
Throughout this work, we will call this sub-sample of Y1 GOLD catalog vetoed by DES GOLD flags and Cuts as \verb|train| sample. BOSS CMASS galaxies in train sample will be called as \verb|train-CMASS| sample, and the rest of sources will be called \verb|train-NoCMASS| sample. The
\verb|train-CMASS| and \verb|train-NoCMASS| samples will be used to train model likelihoods in the next section. 

\subsubsection{The Probabilistic Model}

We build a probabilistic model based on Bayesian statistics as
\bea
p({O \in \rm CMASS}|a_j) = \frac{p(a_j|{ O \in \rm CMASS})~P({\rm O \in CMASS})}{p(a_j)}
\label{eq:model}
\eea
where O stands for a galaxy, and $a_j$ is the $j_{th}$ property of a galaxy has. 
The posterior on the left side $p(O \in {\rm CMASS}|a_j)$ will have a value between 0 and 1 and represents how likely a galaxy is to be a member of CMASS given its observed property $a_j$.
%where $a_j$ is the $j_{th}$ property out of input DES quantities. 
The first term in the right side of the equation, $p(a_j| O \in {\rm CMASS})$ in the numerator is a model likelihood that implies a probability that a CMASS galaxy has a property $a_j$. In other words, a model likelihood can be replaced by a distribution of CMASS galaxy sample as a function of property $a = \{a_0, a_1, ..., a_j, ...\}$ that includes $a_j$ as a sub property. Depending on how many properties used, the term can be a simple one dimensional distribution or a complicated multi-dimensional distribution. 
The prior $P(O \in {\rm CMASS})$ represents the overall probability that an object in an area is a CMASS galaxy. This is simply the fraction of CMASS galaxies in \verb|train| sample, if we assume that CMASS galaxies are uniformly distributed over all sky.
The fraction of clean CMASS galaxies in \verb|train| sample is 1.8\% and thus we use $P(O \in {\rm CMASS}) = 0.018$.
% We simply use this value as a prior. 
%over the all DES region with an assumption that CMASS galaxies are uniformly distributed over all sky. 
The denominator is the distribution of properties $a_j$ over all objects in \verb|train| sample. This thus normalizes the posterior as 
\bea
p(a_j) &=& p(a_j|{O \in \rm CMASS})P({ O \in \rm CMASS }) \\
\nonumber
 & & + ~p(a_j| O \notin {\rm CMASS} )P( O \notin { \rm CMASS} ),
 \label{eq:model_denominator}
\eea
where $p(a_j| O \notin {\rm CMASS} )$ is a model likelihood for non CMASS galaxies and also can be rephrased as a distribution of \verb|train-NoCMASS| sample as a function of input properties. $P( O \notin { \rm CMASS} )$ is the fraction of \verb|train-NoCMASS| sample in \verb|train|.
%
%where $a_j$ is $j_{th}$ bin of DES quantity $a$ that can improve likelihood. 
%The first term in the numerator is a likelihood of a CMASS galaxy having $a_j$ quantity in DES photometry. 
%The second term in the numerator is fraction of CMASS galaxies in train sample. 
%The denominator is distributions of all objects in DES catalog. The analytic form of the denominator is given by
%\bea
%p(a_j) &=& p(a_j|{O \in \rm CMASS})P({ O \in \rm CMASS }) \\
 %& & + ~p(a_j| O \notin {\rm CMASS} )P( O \notin { \rm CMASS} )
%\eea
%that normalizes the posterior. 
%

%\cmt{input colors}
We use a total of four properties for the model. These include two DES colors $G_{\rm DET}-R_{\rm DET}$, $R_{\rm DET}-I_{\rm DET}$, and two DES magnitudes $R_{\rm MOD}$ and $I_{\rm MOD}$. These represent the parameter $a$. 
%The DES quantities selected for parameter $a$ in the model are two colors $G_{\rm DET}-R_{\rm DET}$, $R_{\rm DET}-I_{\rm DET}$, and two magnitudes $R_{\rm MOD}$ and $I_{\rm MOD}$. 
%to mimic counterparts in the SDSS photometry. This hoice is mo \cmt{add detail why}. 
%To mimic $i$ band fiber magnitude in SDSS cut \ref{eq:imag_limit}, we chose \verb|mag_auto|.
%
%: colors \verb|mag_detmodel| $g-r$, $r-i$ and apparent magnitude values  \verb|mag_model r| and \verb|i|.
%We will construct the likelihood for CMASS $p(a_j|{\rm CMASS})$ and the likelihood for non-CMASS $p(a_j|\sim{\rm CMASS})$ in the denominator by deconvolving DES color and magnitude distributions of CMASS with their photometric errors.
%We choose colors \verb|mag_detmodel| $g-r$, $r-i$, $i-z$ and apparent magnitude values  \verb|mag_model r| and \verb|i|.
These two colors are selected as they mirror the SDSS information used for the
 $\dperp$ cut.  The apparent magnitude $I_{\rm MOD}$ is selected reflecting the cut given by \ref{eq:imag_limit}. There is no $r$ band magnitude cut in the CMASS selection criteria, but we decided to include $R_{\rm MOD}$ in order to provide extra information and hope to capture the differences between the SDSS and DES filter bands.
% because 
%\reph{most CMASS galaxies are red luminous galaxies whose spectral feature is the most obvious in $r$ band.}
%Two apparent magnitudes $R_{\rm MOD}$ and $I_{\rm MOD}$ are for substituting for \verb|cmodel i | and \verb|cmodel r| cuts. \verb|cmodel r| is not used in SDSS, but we include this because most CMASS galaxies are red luminous galaxies whose spectral feature is the most obvious in the \verb+r+ band. \cmt{<- confirm this sentence} 
Star-galaxy separation is performed on DES photometry based on the \verb|MODEST == 1| flag \REF{GOLDY1}, therefore we don't apply any further cuts to replace cut \ref{eq:sg} and cut \ref{eq:sg2}. 

The 1D projected distributions of the 4 input DES properties of \verb|train-CMASS| sample are shown in Fig. \ref{fig:hist_cmass_dmass} in blue labeled as 'train'.
The histograms are made by placing galaxies into $100$ evenly spaced bins. It is possible to use these binned histograms directly as a model likelihood but this discrete likelihood heavily depends on sample size and bin size of each property. To avoid the issue, we fit the distributions with a mixture of multi-dimensional Gaussian functions to construct a continuous form of the likelihood function. 
Another advantage of using the continuous form of for the likelihood is that it lets us obtain a 'true' distribution by deconvolving an 'observed' distribution with a given error. The details will be given in the next section. 
%True distribution is free from spatial variance, because spatial variance is mainly caused by photometric error resulted from varying observing conditions. 

%
\subsubsection{Noise deconvolved likelihood}

The true distributions allow us to handle model bias that can possibly happen for the following reasons: %that can happen when the model is defined only in a limited stripe 82 region. 
1. Observed distributions on Stripe82 can be biased compared to SPT.
%cannot represent all DES footprint perfectly because image quality differs from region to region. 
2. Observed distributions can vary drastically with changing observing conditions within the DES SPT region. This implies that applying the same model to the full SPT region cannot be valid.
%2. Applying the same model to all DES footprint without considering spatial variance only adds up more biases.
To overcome these issues, we first obtain true distributions by deconvolving observed distributions from \verb|train| sample with photometric errors on Stripe 82. The true distributions will be convolved with photometric errors of the target region to generate observed distributions that take into account spatially varying photometric conditions.
%the model convolves the true distributions from stripe 82 by photometric errors of the target region to take into account spatially varying photometric condition. 

We used the extreme deconvolution (hereafter XD) algorithm that is built in the python \verb|astroML| package to obtain the underlying true distributions. This algorithm was originally developed by \REF{Bovy} and fits the discrete distributions with a mixture of Gaussian functions. The XD algorithm is a generalized Gaussian-mixture-model approach to density estimation and is designed to reconstruct the error-deconvolved true distribution function common to all samples, even when noise is significant or there are missing data. Starting from the initial guess of Gaussian mixture, the algorithm iteratively calculates likelihood by varying means and sigmas of Gaussian components until it finds the best values of mu and sigma that maximize the likelihood. 

%The XD algorithm fits the distribution to the initial guess of gaussian mixtures and iteratively calculate likelihood by varying means and sigmas of gaussian components until it can found the best values of mu and sigma that maximize the likelihood. Through iterations the gaussian mixtures are deconvolved by given photometric error and approaches to the true distributions of the DES quantities that we should observe if there is no photometric error. 

%\cmt{actual XD running} 
We ran the XD algorithm over \verb|train-CMASS| and \verb|train-NoCMASS| sample separately to obtain a model likelihood for CMASS and the model likelihood for non CMASS in the denominator in equation \ref{eq:model}. Y1 GOLD catalog provides rms errors for different magnitudes as \verb|MAGERR_MODEL| and \verb|MAGERR_DETMODEL| for every source. We derived errors of $G-R$ and $R-I$ colors from the magnitude errors and fed those errors to the XD algorithm with errors of $R_{MOD}$ and $I_{MOD}$ and the chosen input colors in the previous section. 
The XD algorithm in the \verb|astroML| package leaves the initial number of Gaussian Mixture components and likelihood tolerance as a user's choice. \cmt{BIC} gives 8 components for \verb|train-CMASS| sample and 26 components for \verb|train-NoCMASS| sample. The
XD algorithm maximizes the likelihood until an increase of likelihood from the previous iteration becomes less than a given likelihood tolerance. We tested two values for a likelihood tolerance : a moderate value of $10^{-5}$ and an extreme choice $10^{-10}$. Since there was no significant difference found between the two results, we stick to a moderate choice of $10^{-5}$.

In the next section, we will discuss CMASS membership probability that the probabilistic model assigns to each galaxy by using the underlying distributions determined as described in this section. 
%that the probabilistic model that the fitted underlying distributions are plugged in produces for each galaxy and how the CMASS membership probability is used to construct the DES-CMASS sample. 

%\cmt{specific method and re-convolution process} 
%The number of gaussian components for the initial guess is decided by BIC \cmt{add details...} 
%We use DES photometric errors of each color and magnitude that to deconvolve the distribution with. We use \verb|magerr_model[_gri]| and \verb|magerr_detmodel[_gri]|. ( \cmt{add later : descriptions about DES photometric error}). The true distribution should be convolved again with the photometric errors in the target region before multiplied by other factors in the full model. The same procedure should be done for non-CMASS sample to obtain $p(a_j| O \notin {\rm CMASS})$.

\subsubsection{CMASS membership probability}
%\cmt{probability weighting}
Given a set of 4 DES quantities and their photometric errors, the probabilistic model assigns every input galaxy a CMASS membership probability. A similar approach was done in \REF{BovyQuasar}. \REF{BovyQuasar} assigned probabilities to potential SDSS quasars using a flux based model and tested the performance of the model by selecting quasars with a threshold cut $P(\rm 'quasar') > 50 \%$. However the same approach cannot be used for this work since we are not necessarily interested in which objects are the most likely to be CMASS but are instead constructing a sample having similar statistical properties and noise levels as the full BOSS CMASS sample. 

In order to produce a statistical match, the membership probabilities we determine must faithfully reflect the likelihood that an object would be selected into the BOSS CMASS sample based on SDSS imaging. To test this, we looked into the membership probabilities assigned to \verb|train| sample. We binned galaxies in 30 bins by assigned probability and calculated fraction of true CMASS galaxies in each bin. Figure \ref{fig:pc_calib} shows the fraction of true CMASS galaxies in each probability bin. We can easily recognize that the probability that we can find a CMASS galaxy in one bin is same with the value of the assigned probability of the bin. This makes sense because our model is based on the number density distribution of CMASS in color space and the concept of the number density distribution itself is already probability distribution. This test demonstrates that we can either sample a galaxy based on or weight a galaxy by its assigned probability in order to produce a sample that is a statistical match to the BOSS CMASS sample.
%\cmt{It would be good to have more theoretical reason for this than observing cmass fraction directly... } 
%In other words, an assigned probability implies a galaxy in the Y1 Gold catalog to be selected as a DES-CMASS galaxy and the re-sampled galaxies by its assigned probability would have the same CMASS fraction - assigned probability curve and also expected to have the same statistical properties. 

%We applied the model to the full DES SPT region. We weighted each DES Y1 Gold galaxy in the region by its assigned probabilities. 
%Weighted SPT galaxies gives us the exactly same curve of t
%Based on this, we sampled gold galaxies in SPT area along the probability curve. We binned sources into 200 divided probability bins and sampled each bin by the center value of each bin. 
%The majority of sources in DES GOLD catalog are assigned probabilities close to zero. 
%At some threshold, these objects become so unlikely to be CMASS galaxies that keeping them only adds noise to the sample. 
%We carefully tested how the low probability portion of the SPT sample affects the recovered galaxy bias and compared the results to measurements made for the BOSS CMASS SGC data. We removed all galaxies lower than a given probability threshold and measured the clustering for each sample. We found that the galaxy bias becomes stable and safely within the statistical error of CMASS SGC at a threshold of 0.003. We chose 0.01 as our threshold choice. {\bf Include plot? Some statement about why 0.01}
